# Supplementary material for: A-ACT: Action Anticipation through Cycle Transformations
Source: arXiv:2204.00942 source file (2022-04-02)
Supplement: Supplementary file 1 [file 11_additional_results.tex]

% \begin{table}[t]
%     \caption{\textbf{Impact of Past Experience And Future Visualization}}
%     \centering
%     \renewcommand{\arraystretch}{1.35}
%     \begin{tabular}{c|c}
%     \toprule[1.2pt]
%          Methods &  Top-5 Accuracy\\
%     \toprule[1.2pt]
%          RU-LSTM (RGB) & 30.83 \\
%          + PE  & 31.05 \\
%          + FV  & 31.15 \\
%     \toprule[1.2pt]
         
%     \end{tabular}
%     \label{tab:ru_ab}
% \end{table}

% \begin{table}[t]
%     \caption{\textbf{Impact of Cycle Transformation}}
%     \centering
%     \renewcommand{\arraystretch}{1.35}
%     \begin{tabular}{c|c}
%     \toprule[1.2pt]
%          Methods &  Top-5 Accuracy\\
%     \toprule[1.2pt]
%          RU-LSTM (RGB) & 30.83 \\
%          + U-ACT  & \textbf{31.90} \\
%          \hline
%          RU-LSTM (Flow) & 21.42 \\
%          + U-ACT  & \textbf{22.17} \\
%          \hline
%          RU-LSTM (Obj) & 29.89 \\
%          + U-ACT  &  \\
%     \toprule[1.2pt]
         
%     \end{tabular}
%     \label{tab:ru_c}
% \end{table}


% \begin{itemize}
%     \item Action - Our models with different settings - A, B and Cycle at 1s
%     \item Action - Validation set comparison with - A, B and Cycle - Different time steps
%         \item Ablation on Cycle: \textbf{Think before}
%     \item Action - Impact of our modules on other methods like RULSTM + A, B and Cycle
%     \item Procedural Activities dataset: 50Salad or BreakFast. For BreakFast the setup is different - A, B and Cycle
%     \item Multi-possibilities anticipation Action - Multi-Action Anticipation with - A, B and Cycle
    
%     \item Action - Test set SOTA comparison with - A, B and Cycle + Feature Fusion
    
    

%     \item Verb and Noun - SOTA comparison with - A, B and Cycle + Feature Fusion
    

    
% \end{itemize}
